# Supplementary material for: Molecular simulations to investigate the impact of N6-methylation in RNA recognition: Improving accuracy and precision of binding free energy prediction
Source: arXiv:2404.14821 ancillary file (2024-04-23)
Supplement: Supplementary file 1 [file SI.pdf]

# Molecular simulations to investigate the impact of N6-methyation in RNA Recognition: Improving Accuracy and Precision of free energy of binding estimation - Supporting Information

Valerio Piomponi Miroslav Krepl Jiri Sponer Giovanni Bussi

April 22, 2024

## S1 systems

List of systems prepared for this work:

- YHT-RNA (5′- CGACAC-3′) - Used to test metadynamics
- YHT-RNA (5′- CGm$^6$ACAC-3′) - Used for HREX on charges
- YHT-hybridRNA (5′- CG(A-to-m$^6$A)CAC-3′) - Used for AFEC
- ssRNA (5′- CGm$^6$ACAC-3′) - Used for HREX on charges
- ss-hybridRNA (5′- CG(A-to-m$^6$A)CAC-3′) - Used for AFEC
- ss-hybridRNA (5′- CG(A-to-m$^6$A)CAC-3′) with TIP3 water model - Used for AFEC
- 3xYHT-RNA (5′- CGACAC-3′) + alchemical water (SPC\E, TIP3P and OPC)
- 3xBulk water + alchemical water (SPC\E, TIP3P and OPC)

## S2 Lennard-Jones perturbations

In order to investigate to what extent the estimation of the $\Delta\Delta G_{bind}$ can be influenced by adjusting Lennard-Jones (LJ) parametrization, we explored a range of reasonable values for the LJ parameters associated with the hydrogen atoms in the methyl group. In the Amber force-field, methyl group hydrogen atoms are characterized by LJ parameters $\epsilon$ and $\sigma$ values of 0.0657 kJ/mol and 0.2471 nm, respectively. However, for other types of hydrogen atoms, these parameters can fall within the intervals of 0.05-0.13 kJ/mol and 0.2-0.3 nm. We computed $\Delta\Delta G_{bind}$ for parameter values within these defined intervals using a reweighting procedure. The results are summarized in Figure S3. It's worth noting that all the reweighted ensembles considere here exhibit a Kish Size that is at least 10 % the size of the unperturbed ensemble, indicating their statistical significance. We observe lower values of $\Delta\Delta G_{bind}$ when both $\epsilon$ and $\sigma$ are set to low values. However, these perturbations are still insufficient to approach the experimental $\Delta\Delta G_{bind}$, which is 9.9 kJ/mol.

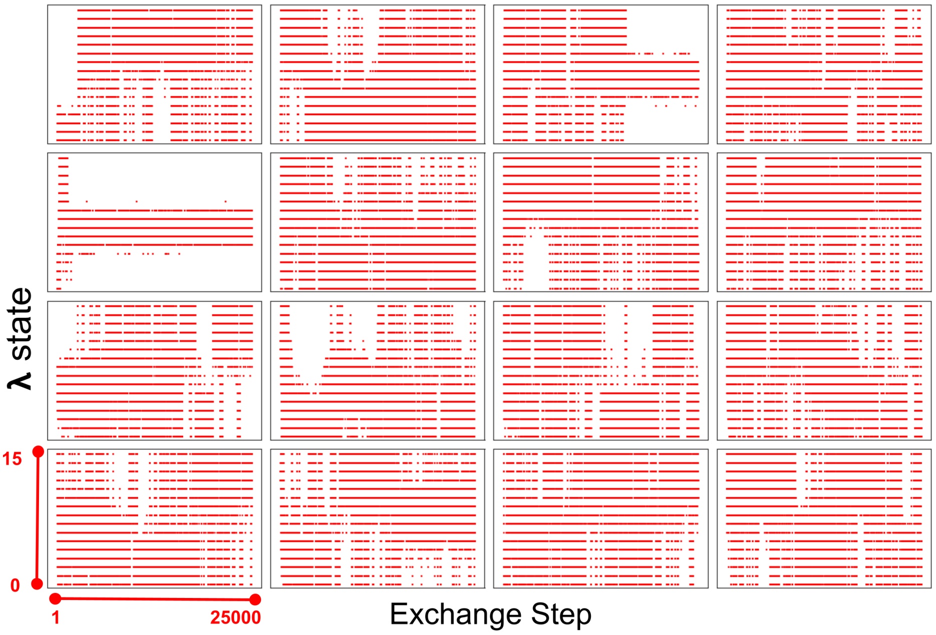


(a)

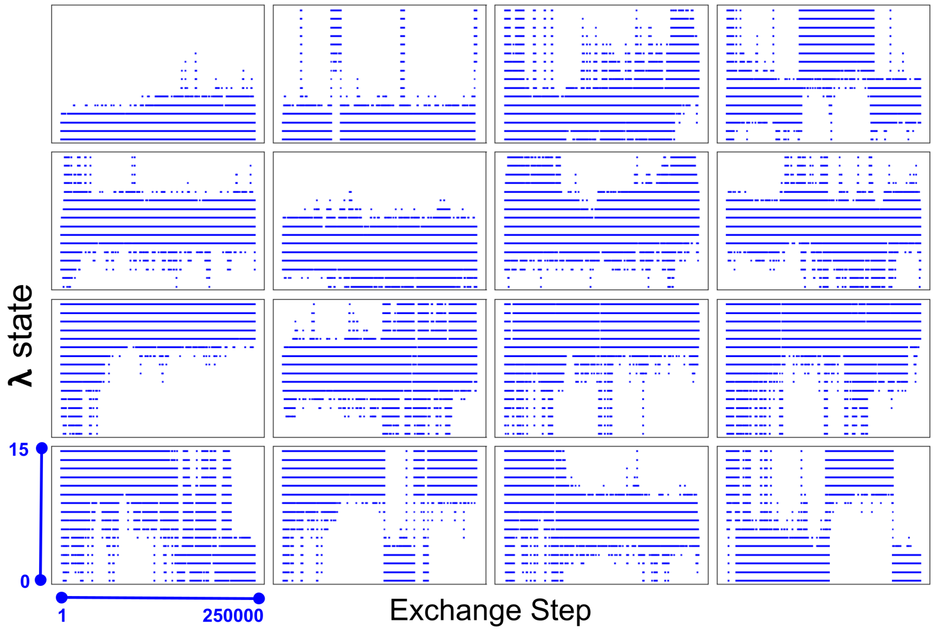


(b)

Figure S1: Exploration of the $\lambda$ ladder in AFEC. Each plot correspond to different continuos demuxed trajectories for the AFEC (a), and for the AFEC+WT-MetaD (b) simulations of the YHT-RNA complex. The Y axis reports the $\lambda$ state at any exchange step in the HREX scheme. Simulations in (b) are 10 times longer than in (a).

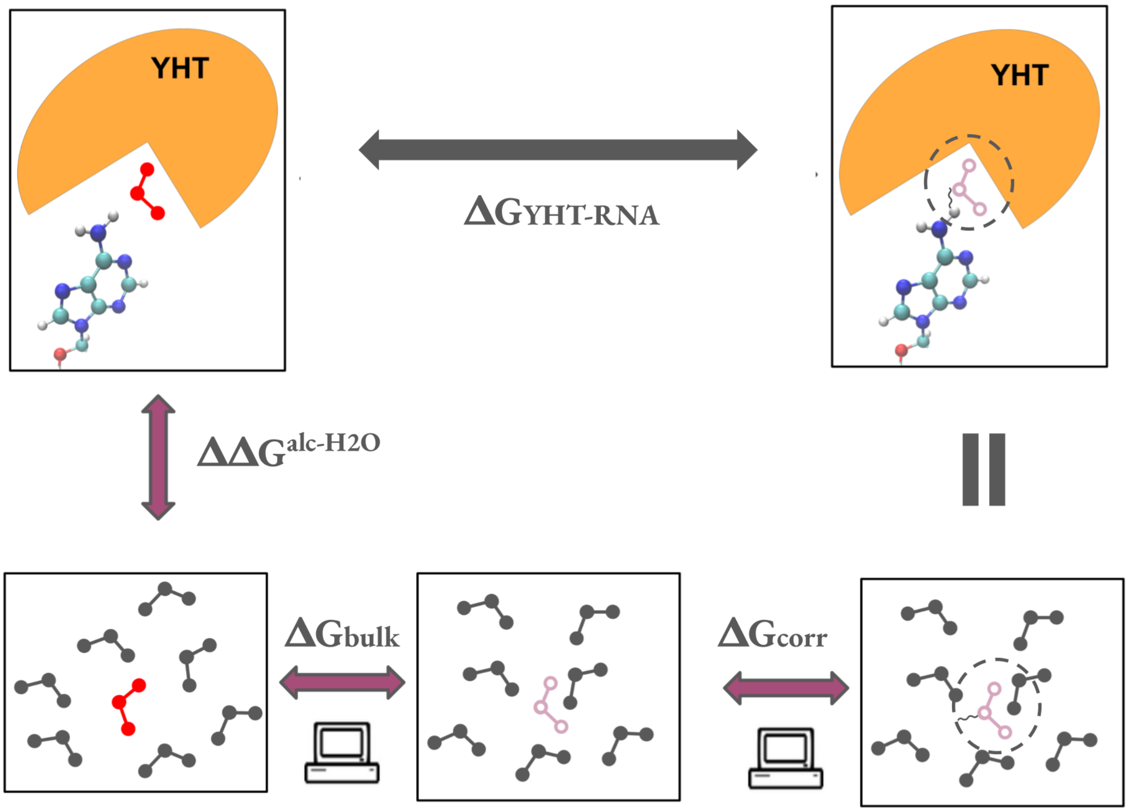


Figure S2: Scheme of the termodynamic cycle used to estimate water molecules preference to stay in buk rather than inside the binding pocket of the YHT-unmethylated RNA complex ($\Delta\Delta G^{alc-H2O}$). $\Delta G^{alc-H2O}_{YHT-RNA}$ is computed through an AFEC consisting in the annihilation of a water molecule inside the binding pocket. During the alchemical simulations, an harmonic restraint is applied on the alchemical water to prevent the decoupled water to leave the binding pocket. $\Delta G^{alc-H2O}_{bulk}$ is computed through an AFEC consisting in the annihilation of a water molecule in bulk with any restraints. The entropic correction $\Delta G^{alc-H2O}_{corr}$ is necessary to keep the relationship between the standard state volume and the accessible space in the binding pocket, and is derived analitically.

| | $\Delta G^{\Delta Q}_{ss}$ | $\Delta G^{\Delta Q}_{com}$ | $\Delta\Delta G^{\Delta Q}_{bind}$ | $\Delta\Delta G^{metad}_{bind}$ | $\Delta\Delta G^{nometad}_{bind}$ |
|---|---|---|---|---|---|
| fit_A-to-Aduri | 50.71 ± 0.10 | 62.37 ± 0.25 | -11.7 ± 0.4 | 8.8 ± 1.6 | 10.2 ± 1.0 |
| fit_A-to-Krepl | -19.78 ± 0.13 | -11.12 ± 0.28 | -8.7 ± 0.3 | 11.8 ± 1.6 | 13.2 ± 0.9 |

Table S1: Impact of $m^6A$ partial charges parametrization on $\Delta\Delta G_{bind}$. First two columns report computed $\Delta G$s for the ssRNA and the YHT-RNA complex with respect to different $m^6A$ charges. Third column ($\Delta\Delta G^{\Delta Q}_{bind}$) report difference in $\Delta\Delta G_{bind}$ with respect to performed simulation with fit_A force-field. Fourth and fifth columns report $\Delta\Delta G_{bind}$ estimated with respect to AFEC with or without WT-MetaD on water displacement. All free energies are reported in kJ/mol.

| | **Aduri** | **fit_A** | **fit6_AC** | **fit5_AC** | **Krepl** |
|---|---|---|---|---|---|
| **N9** | -0.07829 | -0.07829 | -0.07829 | -0.07829 | -0.1719 |
| **C8** | 0.13844 | 0.13844 | 0.13844 | 0.13844 | 0.0631 |
| **H8** | 0.16681 | 0.16681 | 0.16681 | 0.16681 | 0.1973 |
| **N7** | -0.59080 | -0.59080 | -0.59080 | -0.59080 | -0.5652 |
| **C5** | 0.03544 | 0.03544 | 0.03544 | 0.03544 | 0.0152 |
| **C6** | 0.44911 | 0.46801 | 0.53241 | 0.46801 | 0.5597 |
| **N6** | -0.30623 | -0.22923 | -0.28423 | -0.26603 | -0.4756 |
| **H61** | 0.28948 | 0.38888 | 0.31688 | 0.32888 | 0.3232 |
| **C10** | -0.28897 | -0.28467 | -0.31187 | -0.28467 | -0.0774 |
| **H101** | 0.12596 | 0.07536 | 0.09646 | 0.07536 | 0.0774 |
| **H102** | 0.12596 | 0.07536 | 0.09646 | 0.07536 | 0.0774 |
| **H103** | 0.12596 | 0.07536 | 0.09646 | 0.07536 | 0.0774 |
| **N1** | -0.67597 | -0.72167 | -0.65297 | -0.71357 | -0.6604 |
| **C2** | 0.55132 | 0.55132 | 0.55132 | 0.55132 | 0.4636 |
| **H2** | 0.05539 | 0.05539 | 0.05539 | 0.05539 | 0.0865 |
| **N3** | -0.73497 | -0.73497 | -0.73497 | -0.66927 | -0.7027 |
| **C4** | 0.48723 | 0.48723 | 0.48723 | 0.508732 | 0.4589 |

Table S2: Charges for all atoms of the $m^6$A nucleobase for different parametrizations.

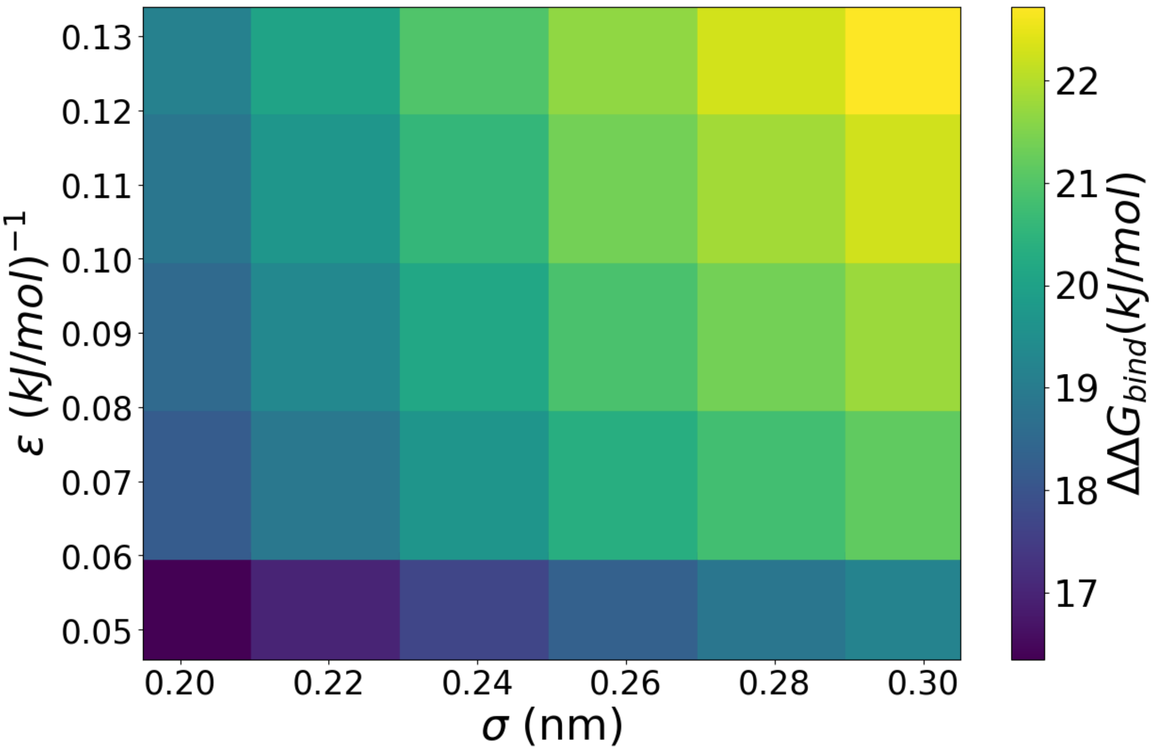


Figure S3: $\Delta\Delta G_{bind}$ computed through reweighting scanning over LJ parameters of the $m^6A$ methyl hydrogens.

| | **Aduri** | | **Aduri+tors** | **fit_A** | | **fit5_AC** | |
|---|---|---|---|---|---|---|---|
| method | BAR | WHAM | WHAM+tors | BAR | WHAM | BAR | WHAM |
| A1 *syn* | 258.24 ± 0.22 | 258.24 ± 0.21 | 258.28 ± 0.21 | 207.19 ± 0.16 | 207.22 ± 0.16 | 237.10 ± 0.20 | 237.00 ± 0.19 |
| A1 *anti* | 260.12 ± 0.12 | 259.95 ± 0.15 | 264.61 ± 0.15 | 213.12 ± 0.20 | 213.29 ± 0.14 | 242.58 ± 0.12 | 242.57 ± 0.23 |
| A2 dup *anti* | 258.85 ± 0.70 | 258.63 ± 0.33 | 263.29 ± 0.33 | 208.32 ± 0.17 | 208.3 ± 0.5 | 241.0 ± 0.6 | 240.93 ± 0.27 |
| A2 dup *syn* | 266.44 ± 0.42 | 266.4 ± 0.4 | 266.4 ± 0.4 | 218.69 ± 0.29 | 218.74 ± 0.31 | 249.2 ± 0.4 | 249.2 ± 0.3 |
| A2 ss *syn* | 257.52 ± 0.31 | 257.54 ± 0.27 | 257.58 ± 0.27 | 206.45 ± 0.28 | 206.50 ± 0.29 | 236.6 ± 0.3 | 236.6 ± 0.4 |
| A3 dup *anti* | 261.56 ± 0.35 | 261.39 ± 0.32 | 266.15 ± 0.32 | 213.10 ± 0.44 | 213.0 ± 0.6 | 244.0 ± 0.3 | 244.1 ± 0.4 |
| A3 dup *syn* | 267.77 ± 0.35 | 267.75 ± 0.30 | 267.79 ± 0.30 | 217.78 ± 0.26 | 217.93 ± 0.24 | | |
| A3 ss *syn* | 257.75 ± 0.24 | 257.80 ± 0.32 | 257.84 ± 0.32 | 206.37 ± 0.29 | 206.31 ± 0.35 | 236.81 ± 0.21 | 236.6 ± 0.4 |
| A4 dup *syn* | 255.06 ± 0.19 | 255.07 ± 0.17 | 255.11 ± 0.17 | 203.76 ± 0.14 | 203.64 ± 0.19 | 234.2 ± 0.5 | 234.19 ± 0.19 |
| A4 ss *syn* | 257.40 ± 0.19 | 257.42 ± 0.18 | 257.46 ± 0.18 | 206.76 ± 0.18 | 206.70 ± 0.17 | 237.30 ± 0.23 | 237.29 ± 0.25 |
| A5 dup *syn* | 256.89 ± 0.11 | 256.80 ± 0.19 | 261.76 ± 0.19 | 206.06 ± 0.25 | 205.89 ± 0.16 | 235.43 ± 0.28 | 235.64 ± 0.23 |
| A5 ss *syn* | 257.56 ± 0.15 | 257.70 ± 0.23 | 257.74 ± 0.23 | 206.65 ± 0.15 | 206.68 ± 0.19 | 236.69 ± 0.15 | 236.6 ± 0.4 |
| B1 dup *anti* | 259.09 ± 0.30 | 259.18 ± 0.21 | 263.94 ± 0.21 | 209.67 ± 0.30 | 209.62 ± 0.38 | 241.5 ± 0.4 | 241.5 ± 0.4 |
| B1 ss *syn* | 257.73 ± 0.25 | 257.60 ± 0.36 | 257.64 ± 0.36 | 205.46 ± 0.14 | 205.37 ± 0.34 | 236.21 ± 0.29 | 236.14 ± 0.28 |
| B2 dup *anti* | 521.6 ± 0.9 | 521.6 ± 0.9 | 530.9 ± 0.9 | 425.24 ± 1.9 | 425.26 ± 1.3 | 486.5 ± 0.9 | 487.0 ± 1.0 |
| B2 ss *syn* | 258.34 ± 0.31 | 258.20 ± 0.35 | 258.24 ± 0.35 | 207.3 ± 0.5 | 206.3 ± 0.5 | 237.6 ± 0.5 | 237.58 ± 0.19 |
| B3 dup *anti* | 518.5 ± 1.0 | 518.6 ± 0.9 | 527.9 ± 0.9 | 420.7 ± 1.0 | 420.7 ± 0.9 | 484.34 ± 0.8 | 484.5 ± 0.9 |
| B3 ss *syn* | 257.74 ± 0.16 | 257.72 ± 0.27 | 257.76 ± 0.27 | 206.77 ± 0.23 | 206.75 ± 0.39 | 236.83 ± 0.10 | 236.85 ± 0.25 |
| B4 dup *anti* | 523.2 ± 1.2 | 523.1 ± 0.5 | 532.4 ± 0.5 | 428.8 ± 1.2 | 428.9 ± 0.9 | 489.7 ± 0.4 | 489.4 ± 1.1 |
| B4 ss *syn* | 257.84 ± 0.45 | 257.85 ± 0.41 | 257.89 ± 0.41 | 206.53 ± 0.29 | 206.72 ± 0.35 | 236.90 ± 0.21 | 236.9 ± 0.4 |
| B5 dup *anti* | 521.9 ± 0.8 | 522.5 ± 0.7 | 531.8 ± 0.7 | 424.0 ± 0.7 | 424.0 ± 1.1 | 487.1 ± 1.0 | 487.0 ± 1.0 |
| B5 ss *syn* | 257.04 ± 0.34 | 257.10 ± 0.43 | 257.14 ± 0.43 | 205.42 ± 0.25 | 205.37 ± 0.23 | 236.63 ± 0.18 | 236.63 ± 0.17 |

Table S3: $\Delta G$s computed through alchemical computations, with different parametrizations and Free Energy methods, reported in kJ/mol. We note that, in addition to the systems required to compute the *syn/anti* balance in the nucleoside (A1) and the effect of methylation in hybridization energies (A2–A5 and B1–B5), this table also reports control results for systems A2 and A3 where the duplex simulation was performed in the unexpected *syn* conformation.

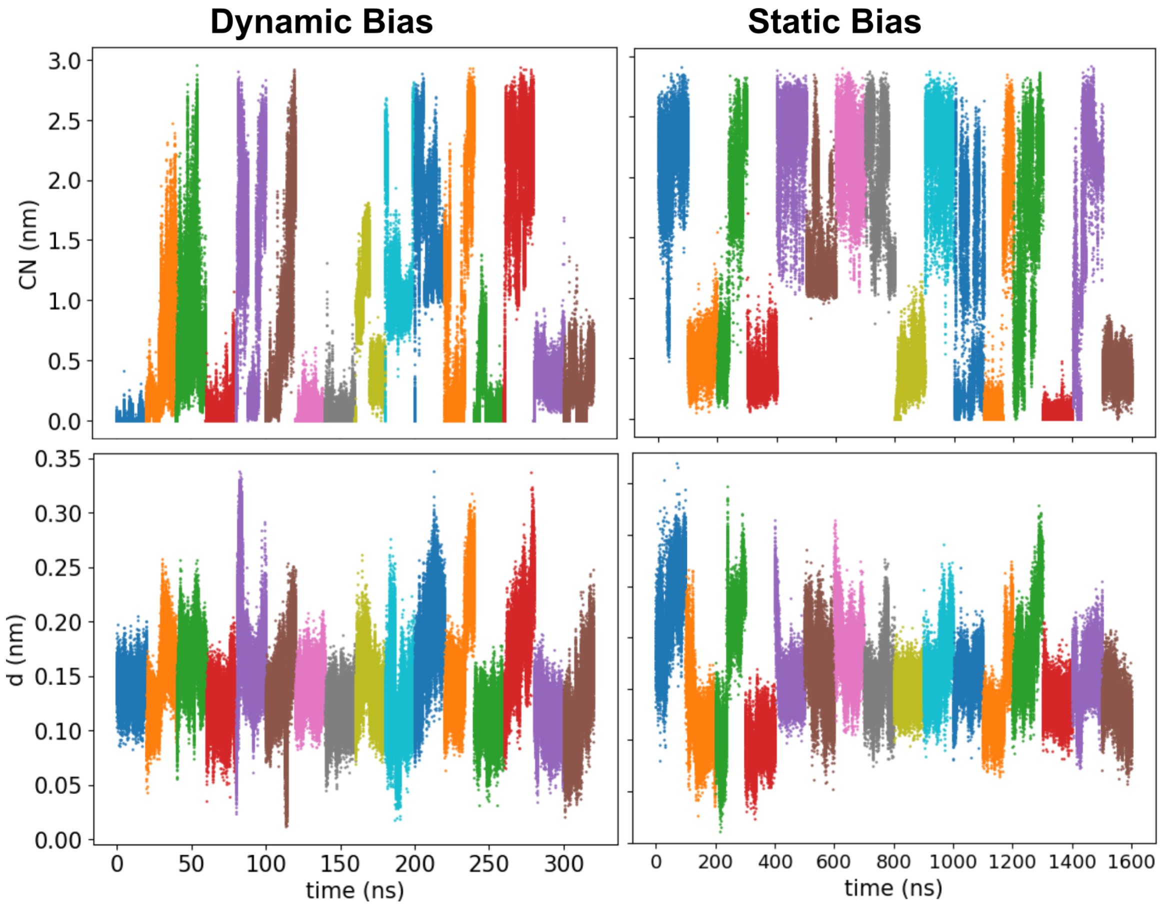


Figure S4: Details of the AFEC+WT-metaD on the YHT-RNA compex. $CN$ (collective variable) and $d$ (control) values along the demuxed trajectories, where each independent trajectory is represented with a different color. Plots on the left correspond to simulations performed with a dynamic bias. Plots on the right correspond to longer simulations performed with a static bias.
